# Supplementary material for: Rewriting and Inductive Reasoning
Source: arXiv:2402.19199 source file (2024-02-29)
Supplement: Supplementary file 1 [file appendix.tex]

\renewcommand{\thesubsection}{\Alph{subsection}}

\subsection{Experimental details}
We show below the theorems only $\vampire_\Sup$, cvc5 or any of the $\vampire_\SymPar$ variants could solve.\medskip\\
{\renewcommand{\arraystretch}{1.2}\small
\begin{tabular}{p{\linewidth}}
\hline
Solved only by $\vampire_\SymPar{}$, $\vampire_\SymParG{}$ or $\vampire_\ParC{}$\\
\hline
$\forall x.\rev(\rev(x))\simeq x$\\
$\forall x,y.\rev(\append(\rev(x),\rev(y)))\simeq\append(y,x)$\\
$\forall x,y.\rev(\append(\rev(x),y))\simeq\append(\rev(y),x)$\\
$\forall x.\rev(\append(\rev(x),\nil))\simeq x$\\
$\forall x.\len(\append(x,x))\simeq\double(\len(x))$\\
$\forall x.\len(\sort(x))\simeq\len(x)$\\
$\forall x.\len(\rev(x))\simeq\len(x)$\\
$\forall x,y.\len(\rev(\append(x,y)))\simeq\plus(\len(x),\len(y))$\\
% hipspec/rev\_equiv\_goal7&$\forall x,y.\qreva(x,\rev(y))\simeq\rev(\append(y,x))$\\
$\forall x,y,z.\nmax(\nmax(x,y),z)\simeq\nmax(x,\nmax(y,z))$(*)\\
$\forall x,y.\nmax(x,y)\simeq\nmax(y,x)$(*)\\
$\forall x,y,z.\nmin(\nmin(x,y),z)\simeq\nmin(x,\nmin(y,z))$(*)\\
$\forall x,y.\nmin(x,y)\simeq\nmin(y,x)$(*)\\
$\forall x.\height(\mirror(x))\simeq\height(x)$\\
$\forall x,y.\cnt(x,y)\simeq\cnt(x,\rev(y))$\\
% isaplanner/goal58&$\forall x,y,z.\drop(x,\take(y,z))\simeq\take(\minus(y,x),\drop(x,z))$\\
$\forall x.\rev(\filter(x))\simeq\filter(\rev(x))$\\
$\forall x.\sorted(\sort(x))$\\
% isaplanner/goal84&$\forall x,y,z.\ztake(x,\zip(y,z))\simeq\zip(\take(x,y),\take(x,z))$\\
$\forall x,y.\len(\rev(\append(x,y)))\simeq(\plus(\len(x),\len(y)))$(**)\\
$\forall x.\len(\append(x,\append(x,x)))\simeq\mult(\len(x),\suc(\suc(\suc(\zero))))$\\
$\forall x,xs.\sort(\append(xs,\cons(x,\nil)))\simeq \insort(x,\sort(xs))$\\
% clam/goal-sg86&$\forall x,y,z.\mult(\expp(x,y),z)\simeq\qexp(x,y,z)$(***)
$\forall x,t.\mtt{ltree}(t)\rightarrow \mtt{ltree}(\mtt{insert\_lheap}(x, t))$
\end{tabular}\medskip\\
\begin{tabular}{p{\linewidth}}
\hline
Solved only by $\vampire_\Sup$\\
\hline
$\forall x,l,r.\insetptree(x,\mtt{join2}(l,r))\leftrightarrow(\insetptree(x,l)\lor\insetptree(x,r))$
\end{tabular}\medskip\\
\begin{tabular}{p{\linewidth}}
\hline
Solved only by cvc5\\
\hline
$\forall x,y.\even(\len(\append(x,y)))\leftrightarrow\even(\plus(\len(x),\len(y)))$\\
$\forall x,l.\neg\mem(x,\delete(x,l))$\\
$\forall i,j,k.\minus(\minus(i,j),k)\simeq\minus(\minus(i,k),j)$\\
$\forall t,l.\fleq(\tsize(\tremoveall(t,l)),\tsize(t))$\\
$\forall x,i.\tsorted(x)\rightarrow\tsorted(\tinsert(x,i))$\\
$\forall x,l.\hasLeftistProperty(x)\rightarrow\len(\qheapsorta(x,l))\simeq\plus(\fhsize(x),\len(l))$\\
$\forall x,y.\hasLeftistProperty(x)\land\hasLeftistProperty(y)\rightarrow \hasLeftistProperty(\merge(x,y))$\\
$\forall x,y.\pref(x,y)\land\len(x)\simeq\len(y)\rightarrow x\simeq y$\\
$\forall x,y.\pref(x,y)\land\len(x)\not\simeq\len(y)\rightarrow\exists e.\pref(\append(x,\cons(e,\nil)),y)$\\
$\forall x,y,z.\equal(x,y,z)\leftrightarrow x\simeq y\land y\simeq z$
\end{tabular}}

% \footnote{(*) does not require inductive reasoning}
% \footnote{(**) using lemma $(= \len \append x (cons y z))) (succ \len \append x z))))$}
% \footnote{(***) using lemma $(= (mult (mult x y) z) (mult x (mult y z)))$}

\subsection{Motivating Example Proof}
{\small
\renewcommand{\arraystretch}{1.2}
\begin{tabular}{l l r}
1.& $\append(\rev(x),\cons(y,\nil)) \simeq \rev(\cons(y,x))$&[\rev.2] \\
2.& $\suc(\len(x)) \simeq \len(\cons(y,x))$&[\len.2]\\
3.& $\cons(y,\append(x,z)) \simeq \append(\cons(y,x),z)$&[\append.2]\\
4.& $\append(\nil,x) \simeq x$&[\append.1]\\
5.& $\len(\rev(\sigma_2))\simeq \len(\sigma_2) $ &[{\sf hyp}] \\
6.& $\len(\rev(\cons(\sigma_1,\sigma_2)))\not\simeq \len(\cons(\sigma_1,\sigma_2)) $ &[{\sf conj}] \\
7.& $\len(\append(\rev(\sigma_2),\cons(\sigma_1,\nil)))\not\simeq \len(\cons(\sigma_1,\sigma_2))\downarrow \len(\rev(\cons(\sigma_1,\sigma_2)))$ &[\DPar 6,1] \\
8.& $\len(\append(\rev(\sigma_2),\cons(\sigma_1,\nil))) \not\simeq \suc(\len(\sigma_2))\downarrow \len(\rev(\cons(\sigma_1,\sigma_2)))$ &[\DPar 7,2] \\
9.& $\len(\append(\rev(\sigma_2),\cons(\sigma_1,\nil))) \not\simeq \suc(\len(\rev(\sigma_2)))\uparrow \suc(\len(\sigma_2))$ &[\UPar 8,5] \\
10.& $\len(\append(\cons(\sigma_3,\sigma_4),\cons(\sigma_1,\nil))) \not\simeq\suc(\len(\cons(\sigma_3,\sigma_4)))$\\
&$\hspace{-1em}\phantom{a}\lor \len(\append(\nil,\cons(\sigma_1,\nil)))\not\simeq \suc(\len(\nil))$ &[\Ind 9] \\
11.& $\len(\append(\sigma_4,\cons(\sigma_1,\nil)))\simeq \suc(\len(\sigma_4))$\\
&$\hspace{-1em}\phantom{a}\lor \len(\append(\nil,\cons(\sigma_1,\nil)))\not\simeq \suc(\len(\nil))$ &[\Ind 9] \\
12.& $\len(\cons(\sigma_3,\append(\sigma_4,\cons(\sigma_1,\nil)))) \not\simeq\suc(\len(\cons(\sigma_3,\sigma_4)))$\\
&$\hspace{-1em}\phantom{a}\lor \len(\append(\nil,\cons(\sigma_1,\nil)))\not\simeq \suc(\len(\nil))\downarrow \len(\append(\cons(\sigma_3,\sigma_4),\cons(\sigma_1,\nil)))$ &[\DPar 10,3] \\
13.& $\suc(\len(\append(\sigma_4,\cons(\sigma_1,\nil)))) \not\simeq\suc(\len(\cons(\sigma_3,\sigma_4)))$\\
&$\hspace{-1em}\phantom{a}\lor \len(\append(\nil,\cons(\sigma_1,\nil)))\not\simeq \suc(\len(\nil))\downarrow \len(\cons(\sigma_3,\append(\sigma_4,\cons(\sigma_1,\nil))))$ &[\DPar 12,2] \\
14.& $\suc(\suc(\len(\sigma_4))) \not\simeq\suc(\len(\cons(\sigma_3,\sigma_4)))$\\
&$\hspace{-1em}\phantom{a}\lor \len(\append(\nil,\cons(\sigma_1,\nil)))\not\simeq \suc(\len(\nil))\downarrow \suc(\len(\append(\sigma_4,\cons(\sigma_1,\nil))))$ &[\DPar 13,11] \\
15.& $\suc(\suc(\len(\sigma_4))) \not\simeq\suc(\suc(\len(\sigma_4)))$\\
&$\hspace{-1em}\phantom{a}\lor \len(\append(\nil,\cons(\sigma_1,\nil)))\not\simeq \suc(\len(\nil))\downarrow \suc(\len(\cons(\sigma_3,\sigma_4)))$ &[\DPar 14,2] \\
16.& $\len(\append(\nil,\cons(\sigma_1,\nil)))\not\simeq \suc(\len(\nil))\downarrow \suc(\len(\cons(\sigma_3,\sigma_4)))$ &[\mtt{EqRes} 15] \\
17.& $\len(\cons(\sigma_1,\nil))\not\simeq \suc(\len(\nil))\downarrow \len(\append(\nil,\cons(\sigma_1,\nil)))$ &[\DPar 16,4] \\
18.& $\suc(\len(\nil))\not\simeq \suc(\len(\nil))\downarrow \len(\cons(\sigma_1,\nil))$ &[\DPar 17,2] \\
19.& $\square\downarrow \len(\cons(\sigma_1,\nil))$ &[\mtt{EqRes} 18]
\end{tabular}}
